# Supplementary material for: Spoofing-Resilient LiDAR-GPS Factor Graph Localization with Chimera Authentication
Source: arXiv:2307.04692 source file (2023-07-10)
Supplement: Supplementary file 1 [file appendix.tex]

\begin{table}[htbp]
\caption{Comparison of RMSE for different methods across spoofing attacks of increasing strength (for 0034)}
    \begin{center}
    \begin{tabular}{|c|c|c|c|}
        \hline
         & \multicolumn{3}{|c|}{\textbf{RMSE (m)}} \\
        \cline{2-4} 
        \textbf{Spoofing rate} & \textbf{\textit{LiDAR Odometry}} & \textbf{\textit{FGO (blind)}} & \textbf{\textit{FGO}} \\
        \hline
        0 m/s      & 70.3 & 1.82 & 1.44 \\
        0.2 m/s    & 70.3 & 3.93 & 4.10 \\
        0.5 m/s    & 70.3 & 9.15 & 8.21 \\
        1.0 m/s    & 70.3 & 18.4 & 5.25 \\
        \hline
    \end{tabular}
    \label{tab:rmse}
    \end{center}
\end{table}

% \begin{table*}[htbp]
% \caption{Per sequence subtable}
%     \begin{center}
%     \begin{tabular}{|c|c|c|c|c|}
%         \hline
%         & 0 m/s & 0.5 m/s & 1.0 m/s & 2.0 m/s  \\
%         \hline
%         Odometry only & 70.3 & 1.82 & 1.44 &  \\
%         Naive FGO     & 70.3 & 3.93 & 4.10 & \\
%         SR FGO        & 70.3 & 9.15 & 8.21 & \\
%         \hline
%     \end{tabular}
%     \label{tab:comp_comparison}
%     \end{center}
% \end{table*}

% \begin{table*}[htbp]
% \caption{Full Comparison}
%     \begin{center}
%     \begin{tabular}{|c|c|c|c|c|}
%         \hline
%         & \multicolumn{4}{|c|}{0018} \\
%         \cline{2-5}  
%         & 0 m/s & 0.5 m/s & 1.0 m/s & 2.0 m/s \\
%         \hline
%         Odometry only (m) & 70.3 & 1.82 & 1.44 &  \\
%         Naive FGO (m)    & 70.3 & 3.93 & 4.10 & \\
%         SR FGO (m)       & 70.3 & 9.15 & 8.21 & \\
%         \hline
%     \end{tabular}
%     \label{tab:full_comparison}
%     \end{center}
% \end{table*}

\begin{table}[htbp]
\caption{Window Size Comparison for Sequence 0027 under 0.2 \si{m/s} Spoofing (computed over 5 Monte Carlo runs)}
    \begin{center}
    \begin{tabular}{|c|c|c|c|c|}
        \hline
         & \multicolumn{4}{|c|}{\textbf{Window size}} \\
        \cline{2-5}         & 20 & 50 & 100 & 200 \\
        \hline
        Mean error          & 7.24 m & 15.3 m & 14.8 m & 13.1 \\
        Max error           & 9.39 m & 22.8 m & 20.4 m & 13.0 \\
        Avg. iteration time & 43.9 m & 134.1 m & 93.2 & 65.2 \\
        \hline
    \end{tabular}
    \label{tab:rmse}
    \end{center}
\end{table}

\begin{table}[htbp]
\caption{Window Size Comparison for Sequence 0027 under 0.2 \si{m/s} Spoofing (computed over 5 Monte Carlo runs)}
    \begin{center}
    \begin{tabular}{|c|c c c c c|}
        \hline
        Window size & 20 & 50 & 100 & 200 & 300 \\
        \hline \hline
        Mean error & x & x & x & x & x \\ 
        Max error & x & x & x & x & x \\
        Avg. iteration time & x & x & x & x & x \\
        \hline
    \end{tabular}
    \label{tab:window_comparison}
    \end{center}
\end{table}

\begin{table}[htbp]
\caption{Performance of our FGO method for spoofing attack of 100s, 1 m/s across the different traces}
    \begin{center}
    \begin{tabular}{|c|c|c|c|c|}
        \hline
         & \multicolumn{4}{|c|}{\textbf{KITTI sequences}} \\
        \cline{2-5} 
                      & 0018 & 0027 & 0028 & 0034 \\
        \hline
        RMSE          & 7.24 m & 15.3 m & 14.8 & 13.1 \\
        Std           & 9.39 m & 22.8 m & 20.4 & 13.0 \\
        Max error     & 43.9 m & 134.1 m & 93.2 & 65.2 \\
        \hline
    \end{tabular}
    \label{tab:rmse}
    \end{center}
\end{table}

\begin{table}[htbp]
\caption{LiDAR odometry mean and max error for each of the KITTI sequences}
    \begin{center}
    \begin{tabular}{|c|c|c|c|c|}
        \hline
         & \multicolumn{4}{|c|}{\textbf{KITTI sequences}} \\
        \cline{2-5} 
                 & 0018 & 0027 & 0028 & 0034 \\
        \hline
        Mean     & 27.9 m & 38.7 m & 46.8 m & 95.0 m \\
        Max      & 107.9 m & 132.3 m & 114.0 m & 273.4 m \\
        \hline
    \end{tabular}
    \label{tab:rmse}
    \end{center}
\end{table}

%% -- Overall FGO algorithm
\begin{algorithm}
%\setstretch{1.2}
\SetAlgoLined
\KwIn{Point cloud $P_k$, GPS measurement $\z_k$}
\KwData{Graph $\G = (\U,\V,\E)$, previous pose $T_{k-1}$, previous point cloud $P_{k-1}$, threshold $\tau$}
\SetKwFunction{ICP}{ICP}
\SetKwFunction{append}{append}
\SetKwFunction{optimize}{optimize}
\SetKwFunction{trim}{trim}
\SetKw{KwTo}{in}
% \newcommand\mycommfont[1]{\ttfamily\textcolor{blue}{#1}}
% \SetCommentSty{mycommfont}
 
\tcp{Run ICP}
$T_{k-1}^k, \Sigma\icp$ = \ICP($P_k,P_{k-1}$)\;
\tcp{Initialize new node using LiDAR odometry pose estimate}
$T_k = T_{k-1}^k T_{k-1}$\;
$\V$.\append(\textsc{Node}($k$, $T_k$))\; 
\tcp{Add LiDAR odometry edge}
$\E$.\append(\textsc{Edge}([$k-1$, $k$], $T_{k-1}^k$, $(\Sigma\icp)^{-1}$))\; 
\tcp{Add GPS factor}
$\E$.\append(\textsc{Edge}([$k$], $\z_k$, $\Omega\gps$))\;
\tcp{Trim graph to window size}
$\G$.\trim($N\window$)\;
\tcp{Optimize}
$\G$.\optimize()\;
\tcp{Compute test statistic}
$q_k = 0$\;
\For{$\e\gps_i$ \KwTo $\E$}{
    $q_k \pluseq (\e\gps_i)\transpose \Omega_i \e\gps_i$\;
} 
\tcp{Check for spoofing}
\If{q_k > \tau}{
    \tcp{Perform mitigation}
    \For{$\e\gps_i$ \KwTo $\E$}{
        $\e\gps_i.\Omega = \zero$\;
    }
}

\caption{Iteration $k$ of Spoofing FGO algorithm}
\label{alg:fgo}
\end{algorithm}
